# Supplementary material for: Machine Learning Enabled Computational Screening of Inorganic Solid Electrolytes for Dendrite Suppression with Li Metal Anode
Source: arXiv:1804.04651 source file (2018-04-12)
Supplement: Supplementary file 1 [file suppinfo.pdf]

# Supporting Information: Machine Learning Enabled Computational Screening of Inorganic Solid Electrolytes for Dendrite Suppression with Li Metal Anode

Zeeshan Ahmad,[†] Tian Xie,[‡] Chinmay Maheshwari,[†] Jeffrey C. Grossman,[‡] and Venkatasubramanian Viswanathan[*,†,¶]

†*Department of Mechanical Engineering, Carnegie Mellon University, Pittsburgh, Pennsylvania 15213, USA*

‡*Department of Materials Science and Engineering, Massachusetts Institute of Technology, Cambridge, Massachusetts 02139, USA*

¶*Department of Physics, Carnegie Mellon University, Pittsburgh, Pennsylvania 15213, USA*

E-mail: venkvis@cmu.edu

## Interface between Li metal and solid electrolyte

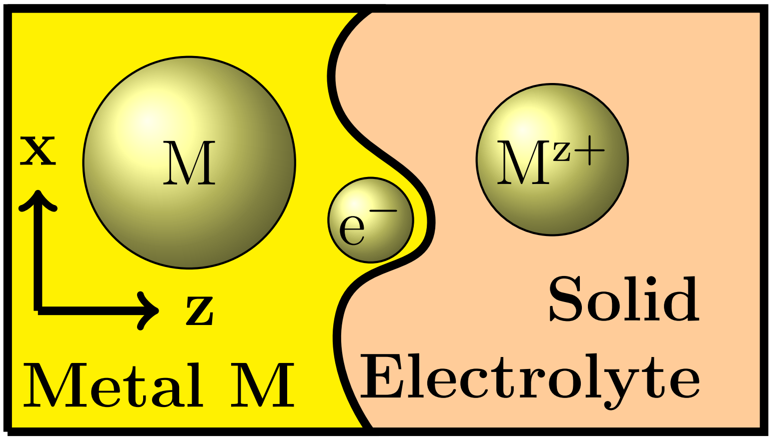


Figure S1: A general 2D interface $z = f(x)$ between Li metal and an inorganic solid electrolyte during electrodeposition.

## Details of the machine learning models

### Isotropic criteria – Crystal Graph Convolutional Neural Network (CGCNN)

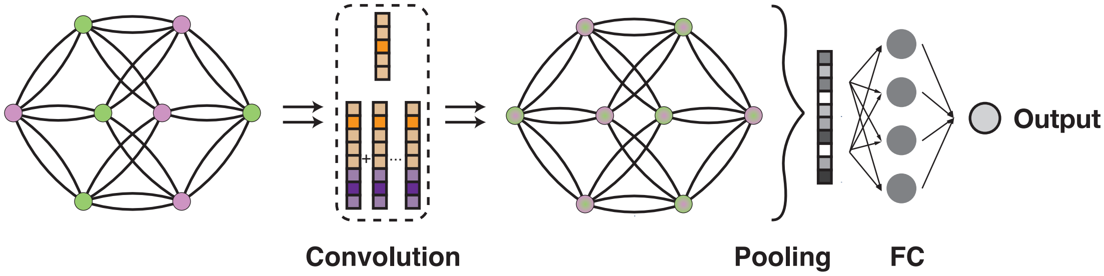


Figure S2: Schematic showing the architecture of CGCNN.

Table S1: Hyper-parameters of the best performing CGCNN model for predicting shear and bulk modulus.

| Property[a] | Shear modulus | Bulk modulus |
|---|---|---|
| Learning rate | $1.0 \times 10^{-2}$ | $2.0 \times 10^{-2}$ |
| Weight decay | $1.0 \times 10^{-4}$ | $1.0 \times 10^{-6}$ |
| Number of convolutional layers | 4 | 4 |

[a] Each model was trained for 1000 epochs, and the learning rate was reduced by 10 fold after 800 epochs.

## Anisotropic criteria

Table S2: List of descriptors used for developing regression model of the elastic tensor. The descriptors have been inspired by Ref.[1] (with some modifications) which used them for ionic conductivity predictions. Some descriptors which were expected to affect only ionic conductivity were removed.

| | |
|---|---|
| 1 | Volume per atom (Å$^3$) |
| 2 | Standard Deviation in Li neighbor count |
| 3 | Standard deviation in Li bond ionicity |
| 4 | Li bond ionicity |
| 5 | Li neighbour count |
| 6 | Li-Li bonds per Li |
| 7 | Bond ionicity of sublattice |
| 8 | Sublattice neighbour count |
| 9 | Anion framework coordination |
| 10 | Minimum anion-anion separation distance (Å) |
| 11 | Volume per anion (Å$^3$) |
| 12 | Minimum Li-anion separation distance (Å) |
| 13 | Minimum Li-Li separation distance (Å) |
| 14 | Electronegativity of sublattice |
| 15 | Packing fraction of full crystal |
| 16 | Packing fraction of sublattice |
| 17 | Ratio of descriptors (4) and (7) |
| 18 | Ratio of descriptors (5) and (8) |
| 19 | Density (g/cc) |

The search space for anisotropic solid-solid interfaces involves low index facets of Li and solid electrolyte. The crystallographic directions $\langle 1\,0\,0\rangle$, $\langle 0\,1\,0\rangle$, $\langle 0\,0\,1\rangle$, $\langle 1\,1\,0\rangle$, $\langle 0\,1\,1\rangle$, $\langle 1\,0\,1\rangle$ and $\langle 1\,1\,1\rangle$ of the solid electrolytes were considered normal to the interface with Li metal anode. We used the elastic tensor of the conventional unit cell obtained from that of the primitive unit cell provided by `materials project`. The new elastic tensor for an arbitrary crystallographic orientation was obtained by rotating the axes and applying the transformation rules.[2]

Using Table S3, one can calculate the total # of interfaces screened over as: # of unique surfaces × # Li surfaces (DFT) + # of unique surfaces × # Li surfaces (predicted) = $2401 \times 4 + 548 \times 3 \times 4 = 16180$.

Table S3: Available # of Li containing compounds in training data for each crystal class. Tetragonal (I) refers to the point groups 4, $\bar{4}$ and 4/m while (II) refers to point groups 4mm, 422, $\bar{4}$2m and 4/mmm. Trigonal (I) refers to point groups 3 and $\bar{3}$ while (II) refers to point groups 32, $\bar{3}$m and 3m.

| Crystal class | # of materials | # unique surfaces[a] |
|---|---|---|
| Cubic | 177 | 3 |
| Hexagonal | 55 | 5 |
| Orthorhombic | 65 | 7 |
| Monoclinic | 63 | 7 |
| Tetragonal (I) | 7 | 6 |
| Tetragonal (II) | 56 | 6 |
| Trigonal (I) | 2 | 5 |
| Trigonal (II) | 44 | 5 |
| Triclinic | 13 | 7 |
| Total | 482 | 2401 |

[a] out of the low index surfaces.

Table S4: Models used for predicting the elastic constants of the cubic crystal class. Hyperparameter optimization was performed using grid-search on `scikit-learn` package.[3] The naming of hyperaparameters is the same as that in `scikit-learn` package.

| Elastic constant | Model | Hyperparameters | |
|---|---|---|---|
| | | Parameter | Value |
| $C_{11}$ | AdaBoost regression | estimators | 500 |
| | | max depth | 100 |
| | | max features | $\log_2$ of total |
| | | minimum samples per leaf | 3 |
| | | minimum samples split | 3 |
| $C_{12}$ | Lasso regression | $\alpha$ | 0.1 |
| $C_{44}$ | Bayesian ridge regression | $\alpha_1$ | $1.0 \times 10^{-5}$ |

Table S5: Surface energies used in calculation of stability parameter.[4]

| Li surface | Surface Energy (J/m$^2$) |
|---|---|
| (1 0 0) | 0.46 |
| (1 1 0) | 0.50 |
| (1 1 1) | 0.54 |
| (2 1 1) | 0.54 |

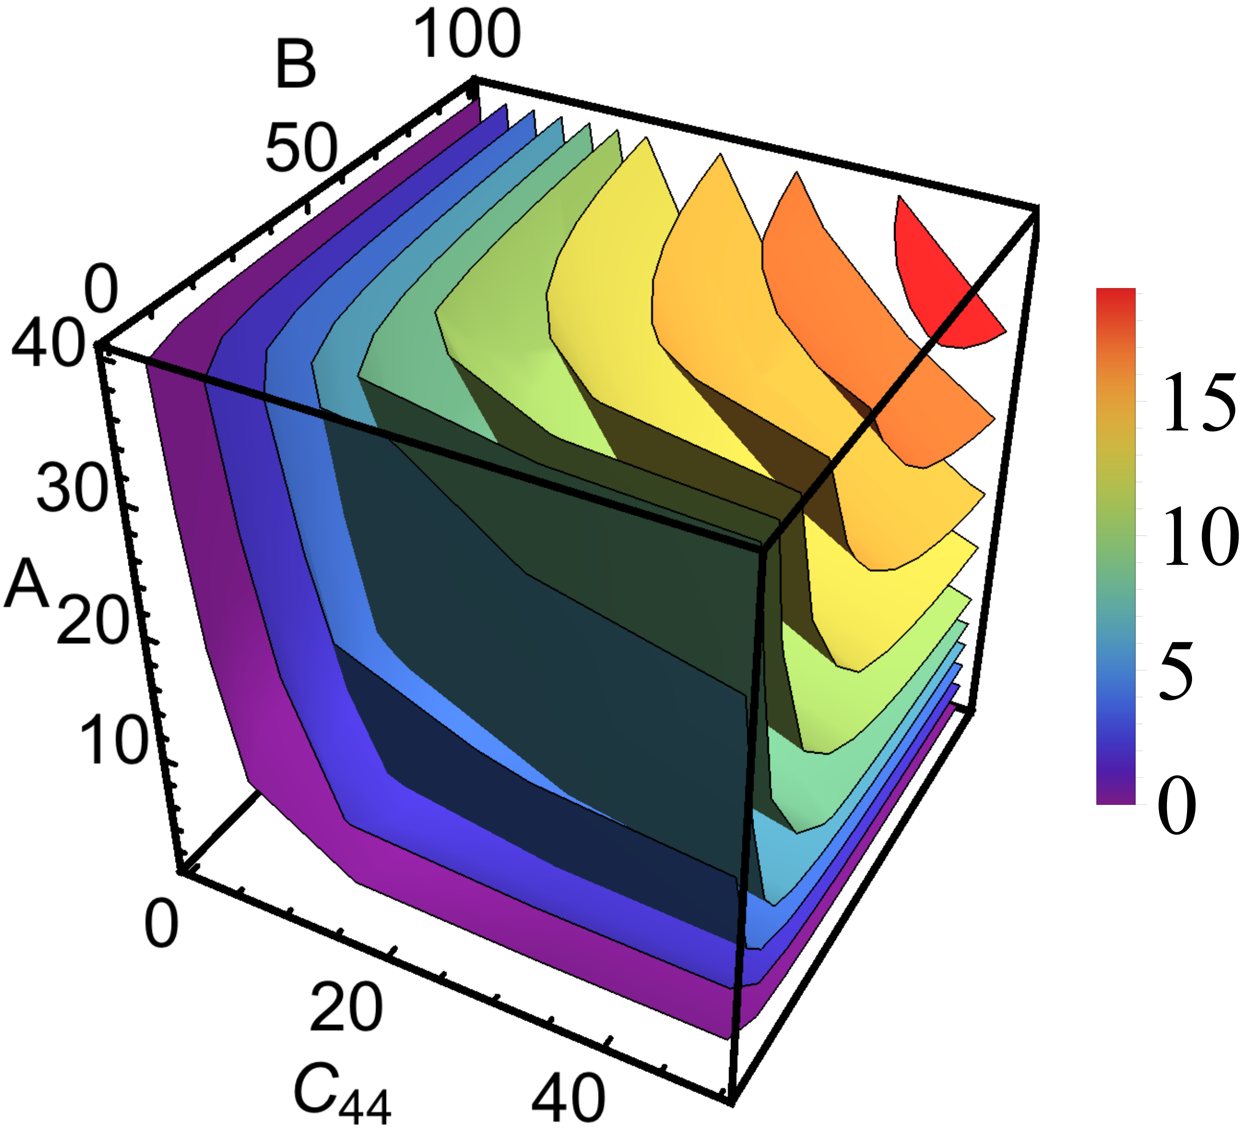


Figure S3: 3D contour plot of the variation of the stability parameter $\chi$ with the eigen values of the elastic tensor for cubic crystal class. The eigen values are $A = C_{11} - C_{12}$, $B = (C_{11} + 2C_{12})/3$ and $C_{44}$. $\chi$ increases as the value of the eigen values is increased. The stability parameter decreases as the material becomes softer i.e. with lower eigen values of the elastic tensor.

# References


(1) Sendek, A. D.; Yang, Q.; Cubuk, E. D.; Duerloo, K.-A. N.; Cui, Y.; Reed, E. J. Holistic computational structure screening of more than 12000 candidates for solid lithium-ion conductor materials. *Energy Environ. Sci.* **2017**, *10*, 306–320.

(2) Ahmad, Z.; Viswanathan, V. Role of anisotropy in determining stability of electrodeposition at solid-solid interfaces. *Phys. Rev. Materials* **2017**, *1*, 055403, DOI: 10.1103/PhysRevMaterials.1.055403.

(3) Pedregosa, F. et al. Scikit-learn: Machine Learning in Python. *J. Mach. Learn. Res.* **2011**, *12*, 2825–2830.

(4) Jain, A.; Ong, S. P.; Hautier, G.; Chen, W.; Richards, W. D.; Dacek, S.; Cholia, S.; Gunter, D.; Skinner, D.; Ceder, G.; Persson, K. A. The Materials Project: A materials genome approach to accelerating materials innovation. *APL Mater.* **2013**, *1*, 011002, DOI: 10.1063/1.4812323.
